# Supplementary material for: Equilibrium and non-equilibrium properties of active matter systems
Source: arXiv:2605.09743 source file (2026-05-10)
Supplement: Supplementary file 1 [file appendix-B.tex]

\chapter{Coarsening dynamics in RBCM with $q$ = 4 and 6}\label{apdxb}

We have shown in Chapter~\ref{chap:Chap4} a true $q$-state discrete version of the Vicsek model. In this Appendix, we show.
